# Supplementary material for: Magneto-optical signature of massless Kane electrons in Cd3As2
Source: arXiv:1604.00038 source file (2016-08-30)
Supplement: Supplementary file 1 [file SI_resubmission.pdf]

# Supplementary materials for
# "Magneto-optical signature of massless Kane electrons in $Cd_3As_2$"


A. Akrap,[1] M. Hakl,[2] S. Tchoumakov,[3] I. Crassee,[4] J. Kuba,[2, 5] M. O. Goerbig,[3] C. C. Homes,[6] O. Caha,[7] J. Novák,[7] F. Teppe,[8] W. Desrat,[8] S. Koohpayeh,[9] L. Wu,[9, 10] N. P. Armitage,[9] A. Nateprov,[11] E. Arushanov,[11] Q. D. Gibson,[12] R. J. Cava,[12] D. van der Marel,[1] B. A. Piot,[2] C. Faugeras,[2] G. Martinez,[2] M. Potemski,[2] and M. Orlita[2, 13, *]

[1] *DQMP, University of Geneva, CH-1211 Geneva 4, Switzerland*
[2] *LNCMI, CNRS-UGA-UPS-INSA, 25, avenue des Martyrs, 38042 Grenoble, France*
[3] *LPS, Univ. Paris-Sud, Univ. Paris-Saclay, CNRS UMR 8502, 91405 Orsay, France*
[4] *GAP-Biophotonics, University of Geneva, CH-1211 Geneva 4, Switzerland*
[5] *CEITEC BUT, Brno University of Technology, 616 00 Brno, Czech Republic*
[6] *CMPMS, Brookhaven National Laboratory, Upton, New York 11973, USA*
[7] *CEITEC MU, Masaryk University, Faculty of Science, 61137 Brno, Czech Republic*
[8] *Laboratoire Charles Coulomb, CNRS, Université Montpellier, 34095 Montpellier, France*
[9] *The Institute for Quantum Matter, The Johns Hopkins University, Baltimore, Maryland 21218, USA*
[10] *Department of Physics, University of California, Berkeley, CA 94720 USA*
[11] *Institute of Applied Physics, Academy of Sciences of Moldova, MD-2028 Chisinau, Moldova*
[12] *Department of Chemistry, Princeton University, Princeton, New Jersey 08544, USA*
[13] *Institute of Physics, Charles University in Prague, 12116 Prague, Czech Republic*


In the Supplementary Materials provided here we discuss the details of the theoretical calculations and data analysis which have been used in the main text.

## BODNAR MODEL – ELECTRONIC BAND STRUCTURE

The model presented for the electronic band structure of $Cd_3As_2$ [1] – employed by Bodnar for the theoretical analysis of previously reported magneto-transport data (Shubnikov-de Haas oscillations) – closely follows the approach proposed by Kildal for another tetragonal semiconductor $CdGeAs_2$ [2].

This model extends the standard Kane model [3], which is widely applied to describe the band structure of zinc-blende (cubic) semiconductors at the $\Gamma$ point and which is based on the exact diagonalization of the $\mathbf{k}\cdot\mathbf{p}$ Hamiltonian, using the finite basis formed from $s$-type ($|S\rangle$) and $p$-type ($|X\rangle$,$|Y\rangle$,$|Z\rangle$) atomic-like valence states:

$$i|S\downarrow\rangle,\ 2^{-\frac{1}{2}}|(X-iY)\downarrow\rangle,\ -2^{-\frac{1}{2}}|(X+iY)\downarrow\rangle,\ |Z\uparrow\rangle,$$
$$i|S\uparrow\rangle,\ 2^{-\frac{1}{2}}|(X+iY)\uparrow\rangle,\ 2^{-\frac{1}{2}}|(X-iY)\uparrow\rangle,\ |Z\downarrow\rangle,$$

where $\uparrow$ and $\downarrow$ refer to the up and down orientation of spin along $z$ axis, respectively.

In this basis, the Hamiltonian may be written, using the notation $k_\pm = (k_x \pm ik_y)/\sqrt{2}$:

$$\hat{H}(\mathbf{k}) = \begin{pmatrix} E_g & P_\perp k_- & -P_\perp k_+ & 0 & 0 & 0 & 0 & P_\parallel k_z \\ P_\perp k_+ & 0 & 0 & 0 & 0 & 0 & 0 & 0 \\ -P_\perp k_- & 0 & -\frac{2}{3}\Delta & \frac{\sqrt{2}\Delta}{3} & 0 & 0 & 0 & 0 \\ 0 & 0 & \frac{\sqrt{2}\Delta}{3} & -(\delta+\frac{\Delta}{3}) & P_\parallel k_z & 0 & 0 & 0 \\ 0 & 0 & 0 & P_\parallel k_z & E_g & P_\perp k_+ & P_\perp k_- & 0 \\ 0 & 0 & 0 & 0 & P_\perp k_- & 0 & 0 & 0 \\ 0 & 0 & 0 & 0 & P_\perp k_+ & 0 & -\frac{2}{3}\Delta & \frac{\sqrt{2}\Delta}{3} \\ P_\parallel k_z & 0 & 0 & 0 & 0 & 0 & \frac{\sqrt{2}\Delta}{3} & -(\delta+\frac{\Delta}{3}) \end{pmatrix}, \quad \text{(S1)}$$

where $E_g$ represents the separation between valence and conduction bands (the band gap), $\Delta$ is the spin-orbit splitting, $\delta$ is crystal-field splitting (due to tetragonal symmetry of $Cd_3As_2$). $P_\parallel$ and $P_\perp$ are (anisotropic) interband matrix elements.

The above Hamiltonian can be rewritten as:

$$\hat{H}(\mathbf{k}) = \hat{H}(\mathbf{k}=0) + P_\perp(k_x\hat{J}_x + k_y\hat{J}_y) + P_\parallel k_z\hat{J}_z, \quad \text{(S2)}$$

The projection of the angular momentum operator $\mathbf{J}$ [4] on an arbitrary direction $\mathbf{n} = (\sin(\theta)\cos(\phi), \sin(\theta)\sin(\phi), \cos(\theta))$, described by spherical coordinates $\theta, \phi$, can be related to $J_z$ by a rotation:

$$\begin{aligned}
\mathbf{J}\cdot\mathbf{n} &= J_x \sin(\theta)\cos(\phi) + J_y \sin(\theta)\sin(\phi) + J_z\cos(\theta) = U_\phi^\dagger (J_x \sin(\theta) + J_z \cos(\theta)) U_\phi \\
&= U_\phi^\dagger U_\theta^\dagger J_z U_\theta U_\phi \ , \qquad \text{(S3)}\\
U_\phi &= \mathrm{diag}\left(1, e^{-i\phi}, e^{i\phi}, e^{i\phi}, e^{i\phi}, e^{2i\phi}, 1, 1\right) \ , \qquad \text{(S4)}\\
U_\theta &= \exp\left(i\theta L\right) \ , \qquad \text{(S5)}\\
L &= \begin{pmatrix}
0 & 0 & 0 & 0 & \frac{i}{2} & 0 & 0 & 0 \\
0 & 0 & 0 & 0 & 0 & 0 & \frac{i}{2} & \frac{i}{\sqrt{2}} \\
0 & 0 & 0 & 0 & 0 & -\frac{i}{2} & 0 & -\frac{i}{\sqrt{2}} \\
0 & 0 & 0 & 0 & 0 & -\frac{i}{\sqrt{2}} & -\frac{i}{\sqrt{2}} & -\frac{i}{2} \\
-\frac{i}{2} & 0 & 0 & 0 & 0 & 0 & 0 & 0 \\
0 & 0 & \frac{i}{2} & \frac{i}{\sqrt{2}} & 0 & 0 & 0 & 0 \\
0 & -\frac{i}{2} & 0 & \frac{i}{\sqrt{2}} & 0 & 0 & 0 & 0 \\
0 & -\frac{i}{\sqrt{2}} & \frac{i}{\sqrt{2}} & \frac{i}{2} & 0 & 0 & 0 & 0
\end{pmatrix} . \qquad \text{(S6)}
\end{aligned}$$

For non-zero $\delta$, this rotation commutes with $\hat{H}(\mathbf{k}=0)$ for any $\phi$ but only at $\theta = 0$. The tetragonal crystal field $\delta$ thus preserves the rotation symmetry along the axis of deformation ($z$-axis) and along this axis the band crossing is maintained.

The Hamiltonian in Eq. (S1) does not allow one to obtain a simple analytical solution for the electronic band structure. Nevertheless, three selected examples of a numerically calculated band structure are presented in Fig. 3 of the main text. The eigenvalues can be analytically found at least at the $\Gamma$ point ($\mathbf{k} = \mathbf{0}$) where we obtain doubly (spin) degenerate bands: $E_1 = E_g$, $E_2^{(\pm)} = -(\Delta+\delta)/2 \pm \sqrt{(\Delta - \delta/3)^2/4 + 2\delta^2/9}$ and $E_3 = 0$. Since $E_3(k_x = 0, k_y = 0, k_z) = 0$ for any $k_z$, the $E_2^{(+)}$ and $E_3$ bands will cross along $k_z$ at zero energy, at $k_z = \pm\sqrt{|E_g|\delta/P_\parallel^2}$.

For $\Delta \gg \delta$, which corresponds well to the studied material ($\Delta = 400$ meV and $\delta = 30$ meV), the above eigenenergies can be expressed as $E_2^+ \approx -2\delta/3$ and $E_2^- \approx -\Delta$. The separation $E_3 - E_2^+ \approx 2\delta/3$ then gives a rough estimate for the energy scale at which the symmetry-protected Dirac electrons appear in $Cd_3As_2$ (Figs. 3a,b in the main text). In contrast, the Kane electrons exist at a considerably larger energy scale, comparable to the strength of the spin-orbit coupling $\Delta$ and thus extend over several hundred meV.

Let us also note that for a negligible anisotropy ($\delta = 0$ and $P_\parallel = P_\perp = P$) and a vanishing band gap ($E_g = 0$), the band structure can be expressed analytically in the limit of infinitely strong ($\Delta \to \infty$) or vanishing ($\Delta = 0$) spin-orbit coupling. The former case has been considered in Ref. 4. The corresponding band structure comprises the doubly-degenerate flat band $E(k) = 0$ and 3D cones $E(k) = \pm v\hbar|k|$ that host the 3D massless charge carries with a velocity of $v = \sqrt{2/3}P/\hbar$ referred to as Kane electrons. In the other limit, for the vanishing $\Delta$, we also obtain a doubly spin-degenerate 3D cone $E(k) = \pm v\hbar|k|$, but with a fourfold degenerate flat band $E(k) = 0$ and a velocity given by $v = P/\hbar$.

## BODNAR/KANE MODEL – OPTICAL RESPONSE AT ZERO MAGNETIC FIELD

In this part we use the Bodnar model and linear response theory to calculate the real part of optical conductivity at $B = 0$,

$$\mathrm{Re}\left\{\sigma_{ii}(\omega)\right\} = \frac{\sigma_0}{\omega}\sum_{l,l'=1}^{8}\int \frac{d^3\mathbf{k}}{(2\pi)^3} \underbrace{\left(f_D(E_l(\mathbf{k})) - f_D(E_{l'}(\mathbf{k}))\right)}_{\text{band occupation}} \underbrace{|c_l^\dagger(\mathbf{k})\nabla_{k_i}H(\mathbf{k})c_{l'}(\mathbf{k})|^2}_{\text{interband coupling}} \underbrace{\delta(\hbar\omega - (E_l(\mathbf{k}) - E_{l'}(\mathbf{k})))}_{\Rightarrow \text{joint density of states}} \qquad \text{(S7)}$$

where $\sigma_0 = \pi e^2/\hbar^2$ and $l, l'$ label the eigenstates of $\hat{H}(\mathbf{k})$ in Eq. (S1). One has the velocity matrix components $\nabla_{k_i}H = PJ_i$ where $i = x, y, z$ labels the Cartesian coordinates and where we consider the experimentally relevant case $P_\perp \approx P_\parallel = P$.

Studying the optical response at relatively high energies ($\hbar\omega \gg \delta$), we may set $\delta = 0$. Any eigenstate $|l, \mathbf{k}\rangle$ can then be related, according to Eq. (S6), to a state of momentum along $z$, $|l, \mathbf{k}\rangle = \hat{U}_\phi^\dagger \hat{U}_\theta^\dagger |l, k_z = |\mathbf{k}|\rangle$, with the corresponding spherical coordinates $\theta, \phi$.

Furthermore, we take $|E_g| \ll \hbar\omega$ and consider $\Delta$ to be sufficiently large so that we project out the states at the energy of $-\Delta$, which are, up to lowest order in $Pk/\Delta$:

$$\begin{pmatrix} 0 \\ 0 \\ \sqrt{2/3} \\ -\sqrt{1/3} \\ 0 \\ 0 \\ 0 \\ 0 \end{pmatrix}, \begin{pmatrix} 0 \\ 0 \\ 0 \\ 0 \\ 0 \\ 0 \\ \sqrt{2/3} \\ -\sqrt{1/3} \end{pmatrix}. \tag{S8}$$

The projected $6 \times 6$ Hamiltonian thus reads:

$$\hat{H}_\infty(\mathbf{k}) \equiv (Q \cdot P)^\dagger \hat{H}(Q \cdot P) = \hat{H}_\infty(\mathbf{k} = 0) + P\mathbf{k} \cdot \hat{\mathbf{J}}_\infty \tag{S9}$$

$$= \begin{pmatrix} 0 & 0 & 0 & 0 & 0 & Pk_- \\ 0 & 0 & 0 & Pk_+ & 0 & 0 \\ 0 & 0 & 0 & \sqrt{\frac{2}{3}}Pk_z & 0 & \frac{1}{\sqrt{3}}Pk_+ \\ 0 & Pk_- & \sqrt{\frac{2}{3}}Pk_z & 0 & -\frac{1}{\sqrt{3}}Pk_+ & 0 \\ 0 & 0 & 0 & -\frac{1}{\sqrt{3}}Pk_- & 0 & \sqrt{\frac{2}{3}}Pk_z \\ Pk_+ & 0 & \frac{1}{\sqrt{3}}Pk_- & 0 & \sqrt{\frac{2}{3}}Pk_z & 0 \end{pmatrix}, \tag{S10}$$

where $k_\pm = (k_x \pm ik_y)/\sqrt{2}$ and

$$Q \cdot P = \begin{pmatrix} 0 & 0 & 0 & 1 & 0 & 0 \\ 0 & 1 & 0 & 0 & 0 & 0 \\ 0 & 0 & 0 & 0 & \frac{1}{\sqrt{3}} & 0 \\ 0 & 0 & 0 & 0 & \sqrt{\frac{2}{3}} & 0 \\ 0 & 0 & 0 & 0 & 0 & 1 \\ 1 & 0 & 0 & 0 & 0 & 0 \\ 0 & 0 & \frac{1}{\sqrt{3}} & 0 & 0 & 0 \\ 0 & 0 & \sqrt{\frac{2}{3}} & 0 & 0 & 0 \end{pmatrix}. \tag{S11}$$

We can use the previous rotation property,

$$\begin{aligned} \mathbf{J}_\infty \cdot \mathbf{n} &= J_{\infty,x}\sin(\theta)\cos(\phi) + J_{\infty,y}\sin(\theta)\sin(\phi) + J_{\infty,z}\cos(\theta) = U_{\infty,\phi}^\dagger (J_{\infty,x}\sin(\theta) + J_{\infty,z}\cos(\theta))U_{\infty,\phi} \\ &= U_{\infty,\phi}^\dagger U_{\infty,\theta}^\dagger J_{\infty,z} U_{\infty,\theta} U_{\infty,\phi} && \text{(S12)} \\ U_{\infty,\phi} &= \mathrm{diag}\left(e^{2i\phi}, e^{-i\phi}, 1, 1, e^{i\phi}, e^{i\phi}\right) && \text{(S13)} \\ U_{\infty,\theta} &= \exp\left(i\theta L^\infty\right) && \text{(S14)} \end{aligned}$$

$$L_\infty = \begin{pmatrix} 0 & 0 & 0 & 0 & i\frac{\sqrt{3}}{2} & 0 \\ 0 & 0 & i\frac{\sqrt{3}}{2} & 0 & 0 & 0 \\ 0 & -i\frac{\sqrt{3}}{2} & 0 & 0 & i & 0 \\ 0 & 0 & 0 & 0 & 0 & \frac{i}{2} \\ -i\frac{\sqrt{3}}{2} & 0 & -i & 0 & 0 & 0 \\ 0 & 0 & 0 & -\frac{i}{2} & 0 & 0 \end{pmatrix}, \tag{S15}$$

and obtain the states $|l, k_z = |\mathbf{k}|\rangle$ from the following rotated Hamiltonian,

$$\hat{H}_{\infty,z}(\mathbf{k}) \equiv U_{\infty,\phi}^\dagger U_{\infty,\theta}^\dagger (Q.P)^\dagger \hat{H}(Q.P) U_{\infty,\theta} U_{\infty,\phi} = \sqrt{\frac{2}{3}} Pk \hat{J}_{\infty,z}. \tag{S16}$$

We find the following three eigenenergies:

$$E_0(\mathbf{k}) = 0, E_\pm(\mathbf{k}) = \pm\sqrt{\frac{2}{3}}Pk, \tag{S17}$$

corresponding to the following six eigenstates:

$$\begin{pmatrix} 1 \\ 0 \\ 0 \\ 0 \\ 0 \\ 0 \end{pmatrix}_{0,1}, \begin{pmatrix} 0 \\ 1 \\ 0 \\ 0 \\ 0 \\ 0 \end{pmatrix}_{0,2}, \frac{1}{\sqrt{2}}\begin{pmatrix} 0 \\ 0 \\ 1 \\ 1 \\ 0 \\ 0 \end{pmatrix}_{+,1}, \frac{1}{\sqrt{2}}\begin{pmatrix} 0 \\ 0 \\ 0 \\ 0 \\ 1 \\ 1 \end{pmatrix}_{+,2}, \frac{1}{\sqrt{2}}\begin{pmatrix} 0 \\ 0 \\ 1 \\ -1 \\ 0 \\ 0 \end{pmatrix}_{-,1}, \text{ and } \frac{1}{\sqrt{2}}\begin{pmatrix} 0 \\ 0 \\ 0 \\ 0 \\ 1 \\ -1 \end{pmatrix}_{-,2}. \tag{S18}$$

Since the energies only depend on $|\mathbf{k}|$, the integration over $\theta, \phi$ in Eq.(S7) leads to the following interband coupling for $\sigma_{xx}(\omega)$

$$\begin{aligned} K^x_{ll'} &= P^2 \int d\theta d\phi \; |\langle l, \mathbf{k}|J_x|l', \mathbf{k}\rangle|^2 = P_\perp^2 \int d\theta d\phi \; |\langle l, k_z = |\mathbf{k}||\hat{U}_\theta \hat{U}_\phi J_x \hat{U}_\phi^\dagger \hat{U}_\theta^\dagger |l', k_z = |\mathbf{k}|\rangle|^2 && \text{(S19)} \\ &= P^2 \int d\theta d\phi \; |\langle l, k_z = |\mathbf{k}||\hat{J}_x \cos(\theta)\cos(\phi) - \hat{J}_y \sin(\phi) + \hat{J}_z \sin(\theta)\cos(\phi)|l', k_z = |\mathbf{k}|\rangle|^2 && \text{(S20)} \\ &= \frac{4\pi P^2}{3}\left(2|\langle l, k_z = |\mathbf{k}|\hat{J}_x|l', k_z = |\mathbf{k}|\rangle|^2 + |\langle l, k_z = |\mathbf{k}|\hat{J}_z|l', k_z = |\mathbf{k}|\rangle|^2\right), && \text{(S21)} \end{aligned}$$

where the commutators $[\hat{L}, \hat{J}_x] = -i\hat{J}_z$, $[\hat{L}, \hat{J}_y] = 0$ and $[\hat{L}, \hat{J}_z] = i\hat{J}_x$ have been used.

In the basis of eigenstates ordered as in Eq. (S18), and adding the two states at the energy of $-\Delta$ states from Eq.(S8) in the last two columns, the interband coupling matrix is, up to the lowest order in $Pk/\Delta$,

$$K^x_{ll'} \approx \frac{4\pi P^2}{3}\begin{pmatrix} 0 & 0 & 0 & \frac{1}{2} & 0 & \frac{1}{2} & 0 & 0 \\ 0 & 0 & \frac{1}{2} & 0 & \frac{1}{2} & 0 & 0 & 0 \\ 0 & \frac{1}{2} & \frac{2}{3} & 0 & 0 & \frac{1}{3} & \frac{1}{6} & \frac{1}{3} \\ \frac{1}{2} & 0 & 0 & \frac{2}{3} & \frac{1}{3} & 0 & \frac{1}{3} & \frac{1}{6} \\ 0 & \frac{1}{2} & 0 & \frac{1}{3} & \frac{2}{3} & 0 & \frac{1}{6} & \frac{1}{3} \\ \frac{1}{2} & 0 & \frac{1}{3} & 0 & 0 & \frac{2}{3} & \frac{1}{3} & \frac{1}{6} \\ 0 & 0 & \frac{1}{6} & \frac{1}{3} & \frac{1}{6} & \frac{1}{3} & 0 & 0 \\ 0 & 0 & \frac{1}{3} & \frac{1}{6} & \frac{1}{3} & \frac{1}{6} & 0 & 0 \end{pmatrix}. \tag{S22}$$

Finally, we obtain and approximate formula for the optical conductivity:

$$\begin{aligned} \mathrm{Re}\left\{\sigma^\infty_{xx}(\omega > 0)\right\} &\approx \frac{\sigma_0}{\omega}\frac{4\pi P^2}{3}\int \frac{k^2 dk}{(2\pi)^3}\left[\delta\left(\hbar\omega - \sqrt{\frac{2}{3}}Pk\right) + \frac{2}{3}\delta\left(\hbar\omega - 2\sqrt{\frac{2}{3}}Pk\right) + \delta\left(\hbar\omega - \Delta - \sqrt{\frac{2}{3}}Pk\right)\right] && \text{(S23)} \\ &\approx \frac{e^2}{4\pi v\hbar}\omega\left[\frac{13}{12} + \theta(\hbar\omega - \Delta)\left(1 - \frac{\Delta}{\hbar\omega}\right)^2\right], && \text{(S24)} \end{aligned}$$

where we have introduced the velocity $v = \sqrt{2/3}P/\hbar$ of Kane electrons in the second line.

The last term of the above expression for conductivity represents a good approximation for $\Delta \ll Pk = \sqrt{3/2}(\hbar\omega - \Delta)$ and its profile fits our experimental data well: (i) it is linear in $\omega$ at low frequencies ($\hbar\omega \ll \Delta$), (ii) it becomes superlinear for $\hbar\omega$ comparable with $\Delta$, (iii) for $\hbar\omega \gg \Delta$ the corresponding slope becomes roughly twice as large as compared to low $\omega$, and (iv) the high frequency part of optical conductivity approaches $\hbar\omega \approx \Delta$ when $\mathrm{Re}\left\{\sigma^\infty_{xx}(\omega > 0)\right\}$ is extrapolated to zero. Let us note that the discontinuity in Eq. (S24) is removed when some disorder as well as finite temperature are considered and the step-like Heaviside function is replaced by some smooth profile. Notice further that, to achieve quantitative agreement, a velocity close to half of the value deduced from magneto-optical data has to be considered, see the main text.

We emphasize that the main feature of the change in the slope of the optical conductivity arises, in the form of the step function, due to the presence of novel excitations available at $\hbar\omega \sim \Delta$. Indeed, the lower cone (green in

Fig. 3b,c of the main text) flattens in response to the hybridization with the spin-orbit-split band (yellow) and contributes at these energies to the optical conductivity. This is a pure band effect that yields roughly a factor of 2 to the optical conductivity. Notice, however, that a change in the velocity also affects the optical conductivity via the density of states, which scales as $v^{-3}$. If we take the Bodnar (or Kane) model literally at high energies, one obtains an asymptotic change in the velocity $\sqrt{2/3}v \to v$, which would in principle lower the density of states and thus the optical conductivity, such that the effect would be less pronounced there. However, this effect is compensated by non-linear corrections to the band dispersion at energies $\hbar\omega \gg \Delta$. These corrections generically lower the band velocity rather than enhance it because the involved wave vectors approach the Brillouin-zone borders. The resulting superlinear behavior in the optical conductivity is clearly visible in the inset of Fig. 1(b) in the main text, in the $0.5\ldots1.5$ eV range. This effect is not included in the present models that arise from a $k \cdot p$ theory in the vicinity of the $\Gamma$ point. We therefore attribute the slope change in the optical conductivity mainly to the above-mentioned accessibility of novel electronic excitations.

## BODNAR MODEL – LANDAU LEVEL SPECTRUM

Here we calculate the Landau level spectrum within the Bodnar model, following the approach of Wallace [5]. Experimentally, we probe the system at relatively high energies, well above the Lifshitz point, where the whole band structure is fairly isotropic and the spectrum depends only weakly on the direction of the magnetic field. Therefore, we only consider the magnetic field applied along the tetragonal [001] axis in our below presented analytical calculations. For the other experimentally explored [112] direction, we show results of numerical calculations only (Fig. S1b).

We employ the standard Peierls substitution $\mathbf{k} \to \mathbf{k} - e\mathbf{A}/\hbar$ in the Hamiltonian Eq.(S1) and search for eigenstates in the form

$$\phi_n = \left( \alpha_{1,+}\phi_n \;\; \alpha_{2,+}\phi_{n+1} \;\; \alpha_{3,+}\phi_{n-1} \;\; \alpha_{4,+}\phi_{n-1} \;\; \alpha_{1,-}\phi_{n-1} \;\; \alpha_{2,-}\phi_{n-2} \;\; \alpha_{3,-}\phi_n \;\; \alpha_{4,-}\phi_n \right), \tag{S25}$$

where $\phi_n = \phi_n(y + p_x l_b^2)e^{ip_x x}$ are the solutions of the harmonic oscillator, and $l_B = \sqrt{\hbar/eB}$ is the magnetic length.

The coefficients are solutions of the following eigenvalue equation:

$$\hat{H}_B\Psi = E\Psi,$$

with $\Psi = (\alpha_{1,+}, \alpha_{2,+}, \alpha_{3,+}, \alpha_{4,+}, \alpha_{1,-}, \alpha_{2,-}, \alpha_{3,-}, \alpha_{4,-})$ and

$$\hat{H}_B = \begin{pmatrix} E_g & \sqrt{n+1}\frac{P_\perp}{l_B} & -\sqrt{n}\frac{P_\perp}{l_B} & 0 & 0 & 0 & 0 & P_\parallel k_z \\ \sqrt{n+1}\frac{P_\perp}{l_B} & 0 & 0 & 0 & 0 & 0 & 0 & 0 \\ -\sqrt{n}\frac{P_\perp}{l_B} & 0 & -\frac{2}{3}\Delta & \frac{\sqrt{2}\Delta}{3} & 0 & 0 & 0 & 0 \\ 0 & 0 & \frac{\sqrt{2}\Delta}{3} & -(\delta+\frac{\Delta}{3}) & P_\parallel k_z & 0 & 0 & 0 \\ 0 & 0 & 0 & P_\parallel k_z & E_g & \sqrt{n-1}\frac{P_\perp}{l_B} & \sqrt{n}\frac{P_\perp}{l_B} & 0 \\ 0 & 0 & 0 & 0 & \sqrt{n-1}\frac{P_\perp}{l_B} & 0 & 0 & 0 \\ 0 & 0 & 0 & 0 & \sqrt{n}\frac{P_\perp}{l_B} & 0 & -\frac{2}{3}\Delta & \frac{\sqrt{2}\Delta}{3} \\ P_\parallel k_z & 0 & 0 & 0 & 0 & 0 & \frac{\sqrt{2}\Delta}{3} & -(\delta+\frac{\Delta}{3}) \end{pmatrix} \tag{S26}$$

the eigenvalues of which are the searched Landau levels.

Since we are interested in sharp spectral features in the magneto-optical response, we now focus on $k_z = 0$, which is the relevant case for Kane/Bodnar electrons at energies well above the Lifshitz point.

In this limit, all Landau levels of Bodnar/Kane electrons, including the fundamental one $n = 1$, become 1D bands dispersing with $k_z$ and implying extrema at $k_z = 0$. These extrema give rise to characteristic singularities in the (joint) density of states, and therefore, to a strongly enhanced response in our magneto-optical measurements. This is in contrast with the fundamental ($n = 0$) levels of 3D Dirac electrons. These levels disperse *linearly* with $k_z$ and for the fundamental CR mode ($n = 0^- \to 1$ and $n = 0^+ \to 1$, see Fig. 4a of the main text) imply rather flat density of states. This yields an essentially featureless magneto-optical response, apart from the low-energy cut-off due to the non-zero Fermi level, which is discussed in the next section.

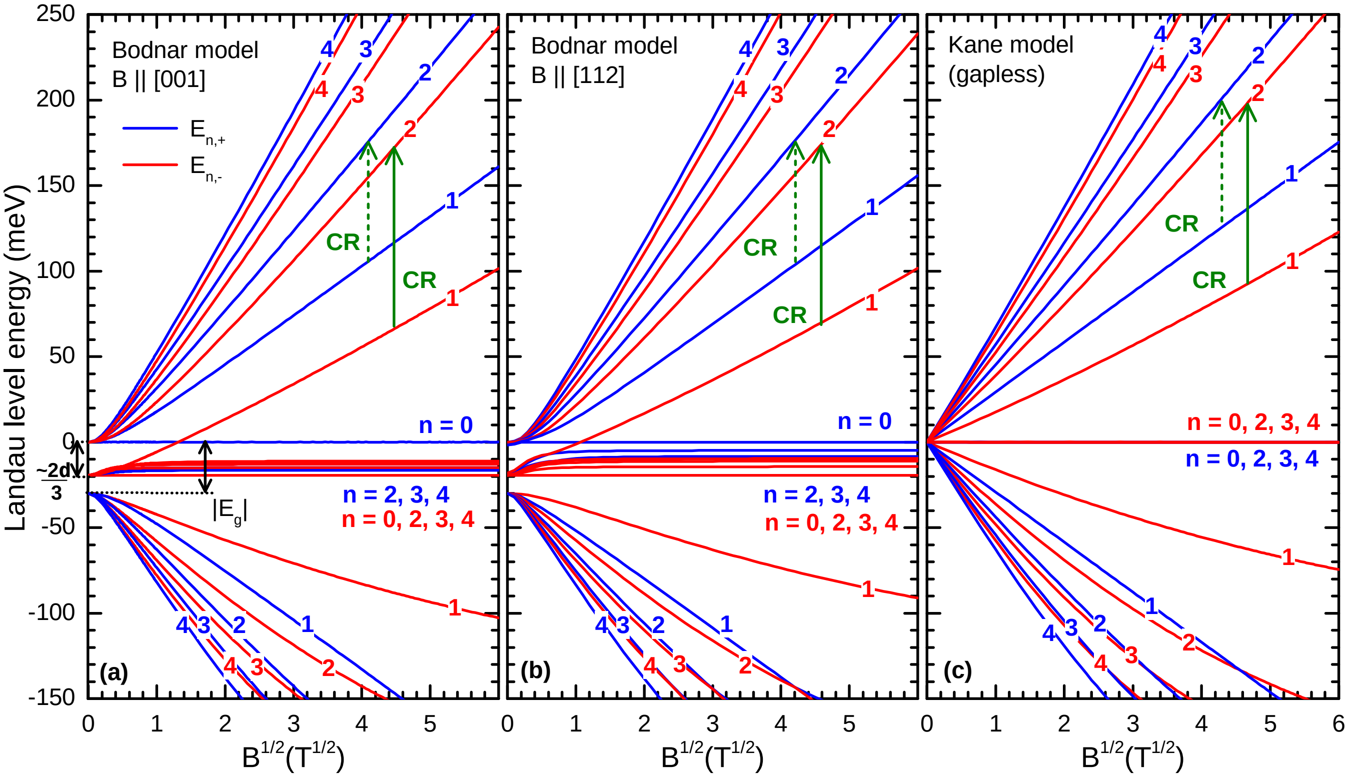


Fig. S1. (a): The LL spectrum (at $k_z = 0$) calculated using the Bodnar model for $\delta = 30$ meV, $E_g = -30$ meV and magnetic field oriented along the [001] direction. (b): The LL spectrum (at $k_{112} = 0$) calculated using the Bodnar model for $\delta = 30$ meV, $E_g = -30$ meV and magnetic field oriented along the [112] direction. (c): The isotropic LL spectrum (at $k = 0$) calculated within the Kane model for $\delta = E_g = 0$. The spin-orbit coupling $\Delta = 400$ meV and the velocity parameter $v = 0.93 \times 10^6$ m/s were used in all the cases. Only LLs at low energies and with indices $n = 0 \dots 4$ were plotted. The blue and red curves correspond to the spin down $E_n^+$ and spin up $E_n^-$ levels, respectively, see the text. The color coding in the part (b) was chosen to reflect the spin projection in high fields (corresponding to the Kane model). At low energies, spin up and down states are strongly mixed for $B \| [112]$. The full vertical arrows correspond to CR modes active when the quantum limit is approached, cf. Fig. 4b in the main text. Notably, the LL spectra calculated within the Bodnar and Kane model become nearly identical for energies high enough, which implies practically the same CR energies. The $n = 0$ and $n = 1$ LLs in the Bodnar model (a) and (b), which cross at the magnetic-field of $B_c \approx 2$ and 1 T, respectively, play the role of zero-mode levels within the Dirac picture ($n = 0^+$ and $n = 0^-$ in Fig. 4a of the main text). At $B < B_c$, these two levels cross as a function of the momentum $k$ along the field direction at the corresponding Dirac points.

For $k_z = 0$, the two $\pm$ subspaces are decoupled, and one can search for solutions of the form ($n \geq 0$)

$$\Psi_{n,+} = \begin{pmatrix} \alpha_{1,+}\phi_{n-1} & \alpha_{2,+}\phi_n & \alpha_{3,+}\phi_{n-2} & \alpha_{4,+}\phi_{n-2} & 0 & 0 & 0 & 0 \end{pmatrix}, \tag{S27}$$

$$\Psi_{n,-} = \begin{pmatrix} 0 & 0 & 0 & 0 & \alpha_{1,-}\phi_{n-1} & \alpha_{2,-}\phi_{n-2} & \alpha_{3,-}\phi_n & \alpha_{4,-}\phi_n \end{pmatrix}. \tag{S28}$$

If $n \geq 2$ the coefficients are solution of

$$\begin{pmatrix} E_g & \sqrt{n}\frac{P_\perp}{l_B} & -\sqrt{n-1}\frac{P_\perp}{l_B} & 0 \\ \sqrt{n}\frac{P_\perp}{l_B} & 0 & 0 & 0 \\ -\sqrt{n-1}\frac{P_\perp}{l_B} & 0 & -\frac{2}{3}\Delta & \frac{\sqrt{2}\Delta}{3} \\ 0 & 0 & \frac{\sqrt{2}\Delta}{3} & -(\delta+\frac{\Delta}{3}) \end{pmatrix} \begin{pmatrix} \alpha_{1,+} \\ \alpha_{2,+} \\ \alpha_{3,+} \\ \alpha_{4,+} \end{pmatrix} = E_{n,+} \begin{pmatrix} \alpha_{1,+} \\ \alpha_{2,+} \\ \alpha_{3,+} \\ \alpha_{4,+} \end{pmatrix} \tag{S29}$$

$$\begin{pmatrix} E_g & \sqrt{n-1}\frac{P_\perp}{l_B} & \sqrt{n}\frac{P_\perp}{l_B} & 0 \\ \sqrt{n-1}\frac{P_\perp}{l_B} & 0 & 0 & 0 \\ \sqrt{n}\frac{P_\perp}{l_B} & 0 & -\frac{2}{3}\Delta & \frac{\sqrt{2}\Delta}{3} \\ 0 & 0 & \frac{\sqrt{2}\Delta}{3} & -(\delta+\frac{\Delta}{3}) \end{pmatrix} \begin{pmatrix} \alpha_{1,-} \\ \alpha_{2,-} \\ \alpha_{3,-} \\ \alpha_{4,-} \end{pmatrix} = E_{n,-} \begin{pmatrix} \alpha_{1,-} \\ \alpha_{2,-} \\ \alpha_{3,-} \\ \alpha_{4,-} \end{pmatrix}. \tag{S30}$$

The lowest Landau levels $n = 0$ and $n = 1$ are special in that many components simply vanish,

1. For $n = 0$, the wave functions have the form

$$\phi_{0,+} = \begin{pmatrix} 0 & \phi_0 & 0 & 0 & 0 & 0 & 0 & 0 \end{pmatrix}, \tag{S31}$$
$$\phi_{0,-} = \begin{pmatrix} 0 & 0 & 0 & 0 & 0 & 0 & \alpha_{3,-}\phi_0 & \alpha_{4,-}\phi_0 \end{pmatrix}. \tag{S32}$$

The three corresponding eigenenergies are

$$E_{0,+} = 0, \tag{S33}$$
$$E_{0,-}^{(\pm)} = -\frac{\Delta+\delta}{2} \pm \sqrt{\left(\frac{\Delta-\delta/3}{2}\right)^2 + 2\delta^2/9}. \tag{S34}$$

The "$-$" coefficients are the solution of

$$\begin{pmatrix} -\frac{2}{3}\Delta & \frac{\sqrt{2}\Delta}{3} \\ \frac{\sqrt{2}\Delta}{3} & -(\delta+\frac{\Delta}{3}) \end{pmatrix} \begin{pmatrix} \alpha_{2,-} \\ \alpha_{4,-} \end{pmatrix} = E_{0,-}^{(\pm)} \begin{pmatrix} \alpha_{2,-} \\ \alpha_{4,-} \end{pmatrix}. \tag{S35}$$

2. For $n = 1$, the wave functions have the form

$$\phi_{1,+} = \begin{pmatrix} \alpha_{1,+}\phi_0 & \alpha_{2,+}\phi_1 & 0 & 0 & 0 & 0 & 0 & 0 \end{pmatrix}, \tag{S36}$$
$$\phi_{1,-} = \begin{pmatrix} 0 & 0 & 0 & 0 & \alpha_{1,-}\phi_0 & 0 & \alpha_{3,-}\phi_1 & \alpha_{4,-}\phi_1 \end{pmatrix}. \tag{S37}$$

The two "+" eigenenergies are

$$E_{1,+}^{(\pm)} = \frac{E_g}{2} \pm \sqrt{\left(\frac{E_g}{2}\right)^2 + \left(\frac{P_\perp}{l_B}\right)^2}, \tag{S38}$$

and the "+" coefficients are solutions of

$$\begin{pmatrix} E_g & \frac{P_\perp}{l_B} \\ \frac{P_\perp}{l_B} & 0 \end{pmatrix} \begin{pmatrix} \alpha_{1,+} \\ \alpha_{2,+} \end{pmatrix} = E_{1,+}^{(\pm)} \begin{pmatrix} \alpha_{1,+} \\ \alpha_{2,+} \end{pmatrix}. \tag{S39}$$

The three "$-$" eigenergies are the solution of the following $3 \times 3$ matrix equation

$$\begin{pmatrix} E_g & \frac{P_\perp}{l_B} & 0 \\ \frac{P_\perp}{l_B} & -\frac{2}{3}\Delta & \frac{\sqrt{2}\Delta}{3} \\ 0 & \frac{\sqrt{2}\Delta}{3} & -(\delta+\frac{\Delta}{3}) \end{pmatrix} \begin{pmatrix} \alpha_{1,-} \\ \alpha_{2,-} \\ \alpha_{4,-} \end{pmatrix} = E_{1,-} \begin{pmatrix} \alpha_{1,-} \\ \alpha_{2,-} \\ \alpha_{4,-} \end{pmatrix}. \tag{S40}$$

The LL spectrum calculated within the Bodnar model has been plotted for $B \parallel [001] \| z$ and for $B \parallel [112]$ into Figs. S1a and S1b, respectively, for parameters considered in the main text ($v = 0.93 \times 10^6$ m/s, $\Delta = 400$ meV, $\delta = 30$ meV and $E_g = -30$ meV). The latter set of LLs was obtained by the full numerical diagonalization of the corresponding $8 \times 8$ Hamiltonian assuming momentum $k_{112} = 0$. In this case, the form of the Hamiltonian does not allow us to facilitate the solution by its separation into two independent $4 \times 4$ Hamiltonians as in the [001] case. The color coding of the spin-up and down projections in Figs. S1b reflects only the approximate spin projection in the limit of high magnetic fields and high energies, when the Bodnar model becomes equivalent to the gapless Kane model. The LL spectrum calculated within the Bodnar model is compared to LLs of gapless Kane electrons ($\delta = E_g = 0$) in Fig. S1c. In all three cases, the fundamental CR mode observed in high magnetic fields is identified as the excitation from $n = 1$ to $n = 2$ LL of the $E_{n,-}$ series and marked by the full vertical arrow. This is because the Fermi energy remains in an electron-doped system pinned to the bottom of the $n = 1$ LL of the $E_{n,-}$ series when the quantum limits is achieved. In high fields, the fundamental CR mode fairly well follows the $\sqrt{B}$ dependence.

Let us now discuss in a greater detail the Landau levels ($n = 0$ and $n = 1$ from the $E_{n,+}$ and $E_{n,-}$ series, respectively), which clearly cross at $B_c \approx 2$ and 1 T in Figs. S1a and S1b, respectively. This crossing is a direct consequence of the band inversion, present in the Bodnar model when $E_g < 0$, and it is also typical of other materials with an inverted band structure, for instance, of topological insulators [6]. The significance of these two crossing levels becomes clear when we look at their particular dispersions with the momentum $k$ along the magnetic field. At $B < B_c$, these

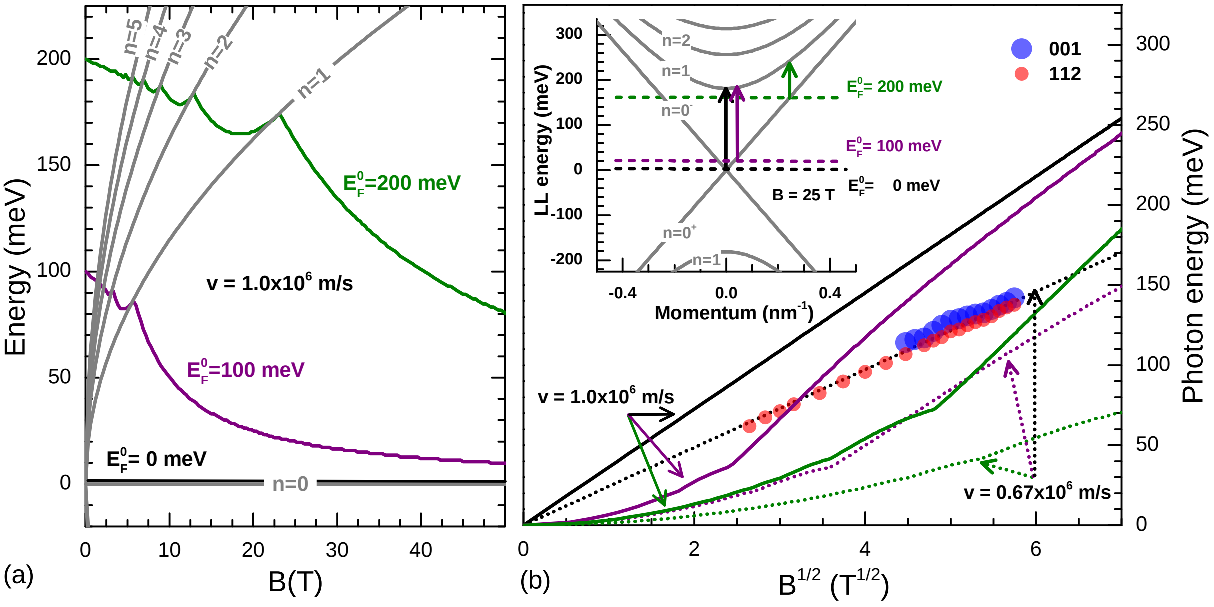


Fig. S2. Part (a): The Fermi energy in a system with 3D massless Dirac fermions ($v = 1.00 \times 10^6$ m/s) as a function of $B$ for the constant carrier density, given by the zero-field Fermi levels: $E_F^0 = 0$, 100 and 200 meV. The Landau level energies, $E_n(k = 0)$ for $n = 0 \ldots 5$, have been plotted for comparison. Part (b): The numerically calculated field dependence of the low-energy absorption edge $L_{0\to1}$ in a system with Landau-quantized 3D Dirac electrons with the fixed carrier concentrations (i.e., field-dependent $E_F$). We have considered two different velocity parameters, $v = 1.00 \times 10^6$ m/s and $v = 0.67 \times 10^6$ m/s (full and dotted lines, respectively), and three different values of the zero-field Fermi energy, $E_F^0 = 0$, 100 and 200 meV (black, violet and green, respectively). The full circles are energies of the experimentally observed fundamental CR modes in the two investigated samples. The inset shows the position of the Fermi energies $E_F(B)$ within the LL spectrum of 3D Dirac electrons at $B = 25$ T, assuming $v = 1.00 \times 10^6$ m/s and three different zero-field chemical potentials $E_F^0$. The vertical arrows mark the excitations corresponding to the low-energy absorption edge $L_{0\to1}$. The experimentally observed (fundamental) CR modes with a clear $\sqrt{B}$ dependence could be, within the picture of 3D massless Dirac electrons, explained only for a vanishing Fermi level (and the velocity $0.67 \times 10^6$ m/s). As we show in the text below, this is at odds with our estimates for the Fermi energy $E_F^{001} \sim 200$ meV and $E_F^{112} \sim 100$ meV for the (001) and (112)-oriented samples, respectively. These estimates are based on the onsets of interband optical absorption (Fig. 1b of the main text) and on the plasma edge splitting at low magnetic fields (Fig. S4).

dispersions imply their crossing in the momentum space for a certain non-zero momentum $k \lesssim k^D$ (and symmetrically for $-k$). At low fields, these specific levels thus play the role of the zero-mode levels of Dirac electrons in $Cd_3As_2$. Within the Dirac picture, these zero-mode LLs (denoted as $n = 0^+$ and $n = 0^-$ in Fig. 4a of the main text) disperse linearly in the vicinity of the Dirac nodes. At magnetic fields above $B > B_c$, the low-energy spectrum loses the character of Dirac-like Landau levels and there a real band gap opens between $n = 0$ and $n = 1$ levels, which is typical of Kane electrons.

The dipole selection rules for inter-LL transitions (at $k_z = 0$) are obtained by evaluating the matrix elements of $\hat{J}_\pm = \hat{J}_x \pm i\hat{J}_y$. In the Faraday configuration (i.e., for radiation propagating along the magnetic field) we obtain:

1. $\Psi_n \to \Psi_{n\pm1}$,

2. transitions between $\Psi_{n,-}$ and $\Psi_{m,+}$ states (so-called spin-flip transitions) are forbidden.

## 3D DIRAC ELECTRONS IN THE QUANTUM LIMIT – OPTICAL RESPONSE

In the main text, based on purely qualitative arguments, we have excluded that the 3D Dirac electrons in $Cd_3As_2$ could be responsible for the specific optical response of $Cd_3As_2$ in high magnetic fields. Here, we extend our considerations and present a quantitative comparison of our cyclotron resonance (CR) data with the response theoretically expected for Landau-quantized 3D Dirac electrons.

Let us first summarize our basic experimental findings. The collected optical and magneto-optical data clearly show the presence of 3D massless charge carriers in $Cd_3As_2$ and indicate high isotropy of the corresponding conical band structure. The zero-field data (onsets of interband absorption and the ratio of plasma energies) provide us with the basic estimates for the Fermi energies $E_F^0 = 50-100$ meV and $100-200$ meV, for the (112)-oriented and (001)-oriented $Cd_3As_2$ samples, respectively. The lower bound is obtained assuming ideal 3D Dirac cones without any electron-hole asymmetry. The real values of $E_F$ most likely approach the upper bound of the above intervals.

The application of high magnetic fields allowed us to observe fundamental CR modes of massless particles in both of the samples. The fundamental CR mode here denotes the situation when electrons are excited from the lowest electronic Landau level (in the conduction band). Let us now (hypothetically) assume that we are indeed dealing with 3D massless Dirac electrons and compare the theoretically expected response with our experimental data.

In the LL spectrum of 3D massless Dirac electrons, $E_n = \pm v\sqrt{2e\hbar Bn + \hbar^2 k^2}$, the fundamental CR mode of electrons corresponds to the excitations from the two $n = 0$ levels to the upper $n = 1$ level, see Fig. 4a in the main text. This fundamental CR mode of 3D Dirac electrons does not imply any singularity in the joint density of states and its only characteristic spectral feature is the low-energy absorption edge at $\mathrm{L}_{0\to1} = \sqrt{v^2 2e\hbar B + E_F^2} - E_F$.

The non-zero Fermi energy implies that this low energy edge cannot follow the $\sqrt{B}$ dependence, and also becomes sensitive to the particular concentration of charge carriers (cf. an analogous situation for Weyl electrons discussed in Ref. 7). Since this behavior is not seen in high-field CR data, we have concluded in the main text that 3D Dirac electrons cannot be responsible the observed magneto-optical response.

Nevertheless, for the Fermi energy $E_F^0$ small enough, the low-energy edge $\mathrm{L}_{0\to1}$ still approaches the $\sqrt{B}$ dependence in the limit of high magnetic fields. Moreover, the carrier concentration stays (most likely) constant with the applied magnetic field, which leads to a continuous drop of $E_F$ with $B$, bringing $\mathrm{L}_{0\to1}$ even closer to the $\sqrt{B}$ dependence. Therefore, to support our main conclusions, here we present a quantitative comparison of our CR data with the theoretically expected edge energy $\mathrm{L}_{0\to1}$, plotted for realistic $v$ and $E_F$ parameters, see Fig. S2.

Let us first focus on the field dependence of $E_F$, under the reasonable assumption that the total electron concentration $N_{\mathrm{total}}$ does not vary with the magnetic field. Such a dependence has been calculated numerically and plotted in Fig. S2a for three selected values of the zero-field Fermi energies $E_F^0 = 0, 100$ and 200 meV, covering thus the range of the Fermi energies relevant for our samples. The velocity parameter was fixed at $v = 1.00 \times 10^6$ m/s. We see that $E_F(B)$ remains roughly constant below the quantum limit, when $E_1(k = 0) < E_F(B)$. Once the quantum limit is achieved, the $E_F(B)$ follows $E_F(B) = N_{\mathrm{total}} v\pi^2\hbar^2/(eB)$.

The expected field-dependence of $\mathrm{L}_{0\to1}$ has been plotted in Fig. S2b. To illustrate that the low-energy edge $\mathrm{L}_{0\to1}$ cannot be used to fit the experimental data by varying the velocity parameter $v$, we have considered its two different values: $v = 1.00 \times 10^6$ m/s and $v = 0.67 \times 10^6$ m/s (full and dotted lines). The former value was chosen to bring the $\mathrm{L}_{0\to1}$ energies close to the experimentally deduced CR energies. The latter value was set to reproduce our experimental data assuming $E_F \equiv 0$ (i.e., $\mathrm{L}_{0\to1} = v\sqrt{2e\hbar B}$). As one may expect, the $\mathrm{L}_{0\to1}$ energy increases with the velocity parameter, but the $\sqrt{B}$ dependence is not recovered for neither of considered velocities, when the experimental estimates of the zero-field Fermi energies are taken into account. Here we recall our realistic estimates of the zero-field Fermi energies in our samples: $E_F^0 \lesssim 100$ meV and $E_F^0 \approx 200$ meV for our (112)- and (001)-oriented samples, respectively, based on our analysis of the zero-field data (Fig. 1a,b in the main text) and also the low-field plasma-edge splitting described below.

This allows us to exclude that the observed response in our high-field magneto-reflectivity measurements could arise from 3D Dirac electrons in $Cd_3As_2$.

## BODNAR VERSUS KANE MODEL – COMPARISON

As mentioned in the main text, the tetragonal nature of $Cd_3As_2$ does not allow the Kane model to be valid down to arbitrarily low energies. Comparing the experimentally observed CR response with the full Bodnar model (Fig. S3) provides us with rough estimates (upper limits) for $\delta$ and $E_g$, which are missing in the simplest gapless Kane model. Convincing agreement between the full Bodnar model and our experimental data (full/open circles versus solid lines in Fig. S3) is obtained when these parameters are taken as large as $E_g = -30$ meV and $\delta = 30$ meV. Let us also note that the origin of the onset $2\delta/3$ appearing for the upper theoretical curve is clarified when confronted with the Landau level spectrum calculated within the full Bodnar model, see Fig. S1a,b.

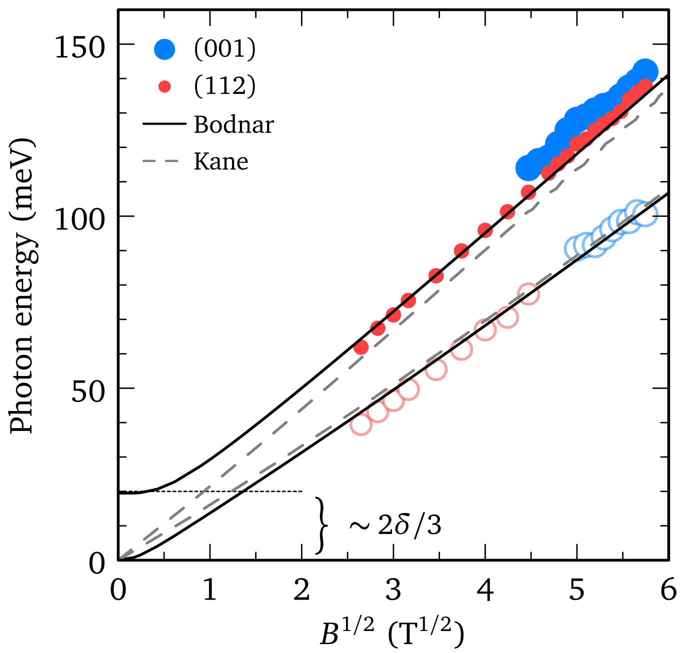


Fig. S3. The experimentally deduced positions of the dominant (full circles) and satellite (open circles) CR modes for both investigated samples. The solid lines show positions expected theoretically within the Bodnar model, assuming $v = 0.93 \times 10^6$ m/s, $\Delta = 400$ meV, $\delta = 30$ meV and $E_g = -30$ meV. The origin of the onset of $2\delta/3$ is explained in the text. For comparison, the dashed lines correspond to the positions of resonances expected within the simplest gapless Kane model (i.e., taking the same parameters, but $\delta = E_g = 0$).

## ANISOTROPY OF VELOCITY – A BASIC ESTIMATE

To quantify the anisotropy of $Cd_3As_2$ based on our magneto-optical data, let us first consider a quasi-classical motion of a charge carrier in a 3D asymmetric conical band. When the magnetic field $B$ is applied, such a particle undergoes a periodic (so-called cyclotron) motion within the plane oriented perpendicular to the field direction. In both momentum and real space, this motion follows an elliptic trajectory characterized by the main axis momenta ($p_\alpha > p_\beta$) and the main axis lengths ($r_\alpha < r_\beta$), respectively. These are connected through relations: $p_\alpha = eBr_\beta$ and $p_\beta = eBr_\alpha$. In addition, the ellipticity of the trajectory may be expressed using the main axes velocities $p_\alpha/p_\beta = v_\alpha/v_\beta$. They correspond to the minimal and maximal in-plane velocities, $v_\beta$ and $v_\alpha$, respectively, achieved by the charge carrier during the cyclotron motion.

When the magnetic field is strong enough, only selected trajectories (Landau levels) become quantum-mechanically allowed. This quantization may be described using the semi-classical Bohr-Sommerfeld rule: $\Phi = BS = (n + \xi)\Phi_0$. While following the cyclotron trajectory, the charge carrier encircles an area, $S = \pi r_\alpha r_\beta$, with a total magnetic flux given by an integer ($n$) multiple of the flux quantum $\Phi_0 = h/e$, corrected by a constant geometrical factor $\xi$. This latter parameter is specific for a given band profile. For a conical band described by the Weyl or Dirac Hamiltonian, it equals zero, but may reach any value between 0 and 1/2 for an arbitrary band [8–10].

Using this Bohr-Sommerfeld rule, we find the energies of Landau levels within an anisotropic conical band,

$$E_n = \pm\sqrt{v_\alpha v_\beta 2e\hbar B(n + \xi) + v_\gamma^2 \hbar^2 k^2}, \tag{S41}$$

where $v_\gamma$ stands for the velocity along the direction of the magnetic field. Even though the details of the LL spectrum depend on the specific value of $\xi$ and on the particular spin-splitting of levels, we may conclude that for $k = 0$ the energies of all LLs and all inter-LL excitations become proportional to the geometrical average of the main axis velocities $\sqrt{v_\alpha v_\beta}$.

The tetragonal symmetry, characteristic of $Cd_3As_2$ and crucial for the presence symmetry-protected 3D Dirac cones at low energies, primarily enters the Bodnar model via crystal field splitting $\delta$. In addition, it may also give rise to an anisotropy of the in-plane and out-of-plane interband matrix element $P_\parallel \neq P_\perp$. Well above the Lifshitz point

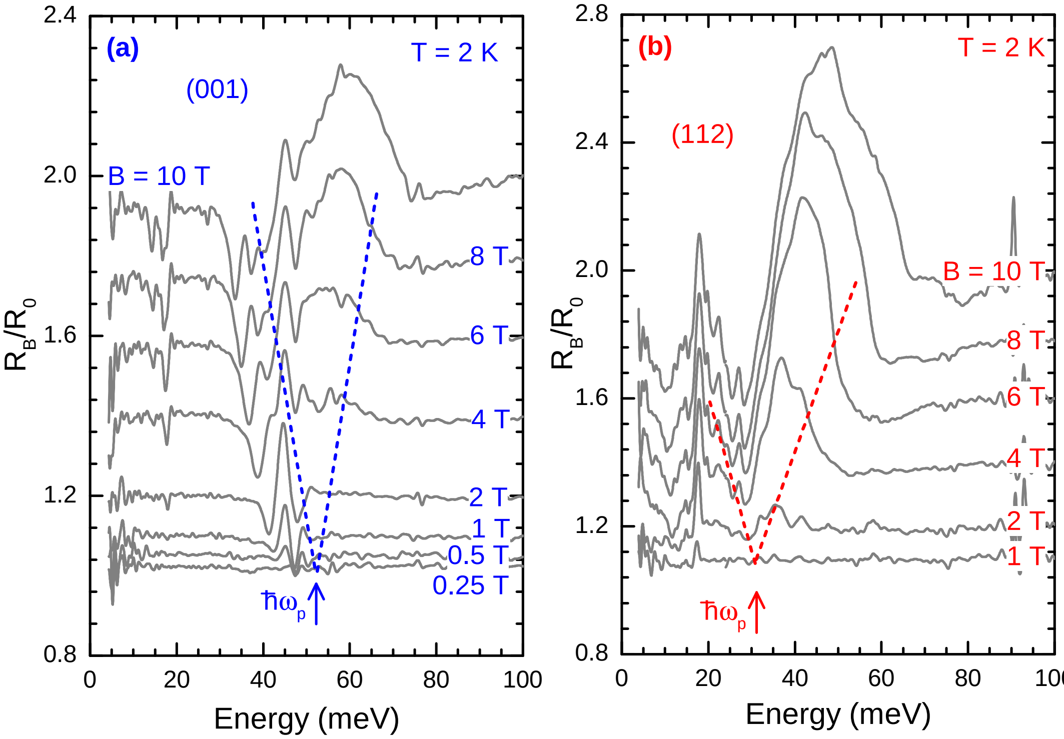


Fig. S4. The splitting of the plasma edge at low magnetic fields as seen in the relative magneto-reflectivity spectra of (001) and (112) sample in the part (a) and (b), respectively. The position of the upper and lower branch is roughly shown by the dashed lines. The sharp features in the spectra are likely due to a thin depletion layer on the surface of samples, see Ref. 12.

in $Cd_3As_2$, i.e., for energies $\Delta \gg |E(k)| \gg \delta$, the Kane electron anisotropy is determined mainly by the interband coupling constants. These can be conveniently expressed using in-plane and out-of-plane velocities, $v_\parallel = \sqrt{2/3}P_\parallel/\hbar$ and $v_\perp = \sqrt{2/3}P_\perp/\hbar$. A rough estimate for the ratio of these velocities, $v_\perp/v_\parallel$, can be obtained from the fairly small, but still present, difference in the energies of the fundamental CR modes, $\alpha = \omega_c^{001}/\omega_c^{112} \sim 1.03$, obtained on samples with the (001)- and (112)-oriented facets. Both these modes evolve with a nearly perfect $\sqrt{B}$ and thus correspond to inter-LL excitations at $k = 0$, which makes them proportional to the geometrical average of the main axis velocities, following Eq. S41.

For the (001)-oriented sample, with the cyclotron motion within an isotropic plane, the CR energy scales linearly with the in-plane velocity, $\omega_c^{001} \propto \sqrt{v_\parallel v_\parallel} = v_\parallel$. A more complex result is obtained for the (112)-oriented sample, since the (112)-plane is not isotropic. Assuming that the lattice constants satisfy $a = b = c/2$ (practically fulfilled in $Cd_3As_2$ [11]), the (112) crystallographic direction becomes equivalent to (1,1,1) direction in the momentum space. The corresponding main axis velocities, in the plane perpendicular to the magnetic field, read $v_\parallel$ and $\sqrt{(v_\parallel^2 + 2v_\perp^2)/3}$, which implies $\omega_c^{112} \propto \sqrt[4]{v_\parallel^2(v_\parallel^2 + 2v_\perp^2)/3}$.

The above formula allows us to express the velocity ratio $v_\perp/v_\parallel$ using only the experimentally determined parameter $\alpha = 1.03$,

$$\frac{v_\perp}{v_\parallel} = \sqrt{\frac{1}{2}\frac{3-\alpha^4}{\alpha^4}} \approx 0.9.$$

## SPLITTING OF PLASMA EDGE AT LOW MAGNETIC FIELDS

The plasma edge in reflectance spectra is characteristic of solids with a non-zero charge carrier density and becomes profoundly modified when a strong enough magnetic field is applied. At relatively low magnetic fields, when the

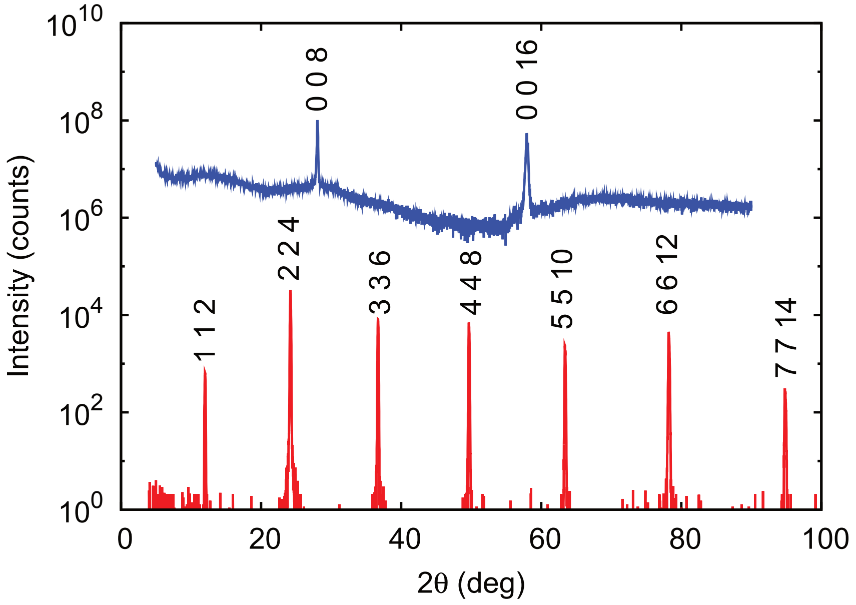


Fig. S5. Symmetric x-ray diffraction scans taken on the (001)- and (112)-oriented samples (top and bottom curve, respectively). The observed Bragg reflections indexed according to the $Cd_3As_2$ crystal structure reported in Ref. 11 are in agreement with the anticipated surface orientations of the respective samples.

motion of charge carriers is still described by laws of classical mechanics ($\omega_c\tau \lesssim 1$), the standard magneto-plasma theory [13] implies that the plasma edge splits into two branches separated by the cyclotron energy, $\hbar\omega_c = eB/m$. In systems with massless charge carriers, the cyclotron mass increases linearly with the Fermi energy, $m = E_F/v^2$.

The field-induced splitting of the plasma edge has been observed in the response of both investigated $Cd_3As_2$ samples, see Fig. S4, where the relative magneto-reflectivity spectra have been plotted at low magnetic fields ($B \leq 10$ T). The position of the upper and lower branches of the split plasma edge are approximately shown by dashed lines, which allow us to set rough estimate for the cyclotron energy in our samples. Notably, the observed splitting is significantly higher for the (112)-oriented sample, which is significantly less doped as compared to the (001)-oriented sample and reflects thus the effective cyclotron mass increasing with the carrier concentration.

In numbers, the splitting of the plasma edge in the (001)-oriented and (112)-oriented sample is estimated to $\sim$3 and $\sim$5 meV/T, which implies the effective mass of $m_{001} \approx 0.04m_0$ and $0.025m_0$, respectively. These values are in rather good agreement with the cyclotron masses $m_{001} = E_F^{001}/v^2 = 0.04m_0$ and $m_{112} = E_F^{112}/v^2 = 0.02m_0$ expected when the parameters deduced from our other optical and magneto-optical data are considered: $v \approx 0.93 \times 10^6$ m/s, $E_F^{001} \approx 200$ meV and $E_F^{112} \approx 100$ meV.

However, we emphasize that the presented estimate of the effective masses is very rough. More precise analysis of the plasma edge splitting is challenging due to an additional series of fairly sharp resonances in the magneto-reflectivity spectra. These are in particular strong in the response of the (001)-oriented sample, see Fig. S4a. Such features have been observed in previous (low-field) magneto-reflectivity experiments performed on $Cd_3As_2$ [12] and interpreted as the response of a thin depletion layer on the surface. Their appearance in the magneto-reflectivity spectra correlates with the fine structure of the zero-field plasma edge, see Fig. 1a in the main text, present around the energy of 35 and 50 meV in the spectra of the (112)- and (001)-oriented samples, respectively.

## SAMPLE SURFACE ORIENTATION

The surface orientations of the two reported $Cd_3As_2$ samples were confirmed using the x-ray diffraction (XRD). We measured symmetric XRD scans, where the scattering vector is parallel to the sample surface normal and, thus, the lattice planes parallel to the sample surface are probed. Resulting diffractograms are shown in Fig. S5 for both samples. The measured Bragg reflections were indexed according to the crystal structure reported in Ref. 11. Reflection series

$h\,h\,2\cdot h$ and $0\,0\,4\cdot l$ observed for the (112)- and (001)-oriented samples, respectively, uniquely confirm the orientation of the sample surface facets.

## MAGNETO-REFLECTIVITY SPECTRA – ADDITIONAL DATA AND ANALYSIS

As discussed in the main text, the dominant CR mode observed in the magneto-reflectivity response of both studied $Cd_3As_2$ samples is likely accompanied by a weak satellite CR line at lower photon energies (Fig. 3 of the main text). Here we provide additional data from the (112)-oriented sample and the detailed data analysis of the high-field data taken on the (001)-oriented sample to support the existence of this satellite line.

In the response of the (112)-oriented sample, the satellite line is observed at relatively low magnetic fields. This allows us to identify this CR mode also in low-field data obtained on this sample. These were collected using a superconducting coil and are characterized by a significantly lower noise level. In Fig. S6, we show both low- and high-field spectra (the latter are shown in the main text) in a form of false color plots. The satellite line, $n = 1^{\downarrow} \rightarrow 2^{\downarrow}$, is very visible at ∼9 T, slightly below its theoretical position as calculated using the Bodnar model (dashed line).

However, let us stress that the purpose of these color plots is to show the existence the spectral feature associated with the satellite line, not to show its exact position. These positions are in the magneto-reflectivity experiments not related to particular minima or maxima in $R_B/R_0$ curves, but instead, they are associated with the corresponding points of inflections in the spectra. Naturally, the points of inflection are not clearly seen in this type of plots. We also note that different color scales used for low- and high-field data in Fig. S6.

The satellite line $n = 1^{\downarrow} \rightarrow 2^{\downarrow}$ was observed also in the response of the (001)-oriented sample. Nevertheless, due to a higher electron density, it emerges only in high magnetic fields for which no data from a superconducting coil (with a reduced noise) are available. The position of this satellite line was extracted using procedure visualized in Fig. S7 for three selected magneto-reflectivity spectra. The high-field $R_B/R_0$ curves (grey circles) were fitted using a high-order polynomial (red curves). The energies of the resonances, associated with the corresponding points of inflections, were then read as the corresponding minima in the first derivative of the polynomial fit (blue curves).

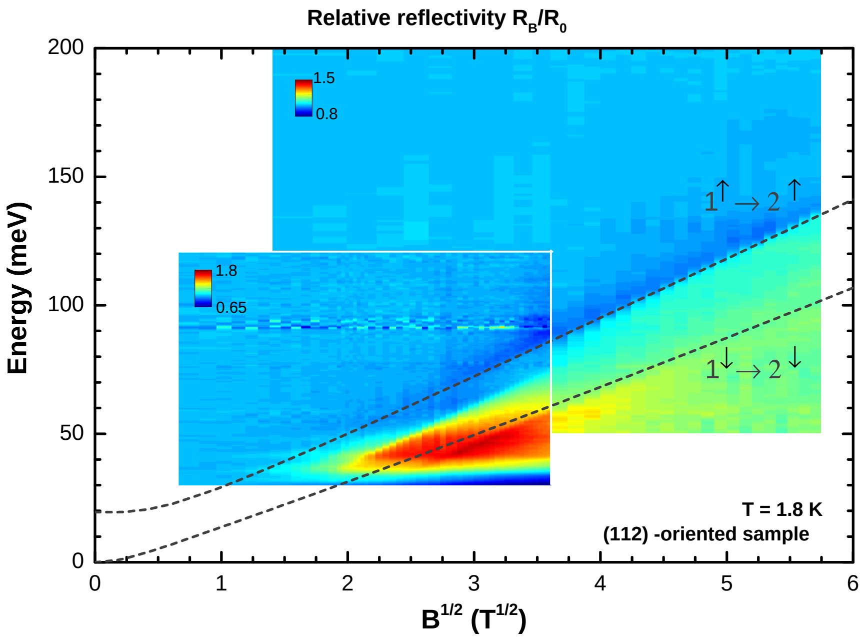


Fig. S6. False color plots of relative magneto-reflectivity $R_B/R_0$ measured on the (112)-oriented sample at low and high magnetic fields, using superconducting ($B \leq 13$ T) and resistive ($B \leq 33$ T) coils, respectively. The dashed lines correspond to the theoretical positions of $n = 1^{\downarrow} \rightarrow 2^{\downarrow}$ and $n = 1^{\uparrow} \rightarrow 2^{\uparrow}$ resonances, predicted using Bodnar model with parameters considered in the main text: $v = 0.93\times10^6$ m/s, $E_g = -30$ meV, $\delta = 30$ meV and $\Delta = 400$ meV. Note the different energy scale used for the low- and high-field data. The weak satellite line ($n = 1^{\downarrow} \rightarrow 2^{\downarrow}$ resonance) is visible slightly below the theoretical curves.

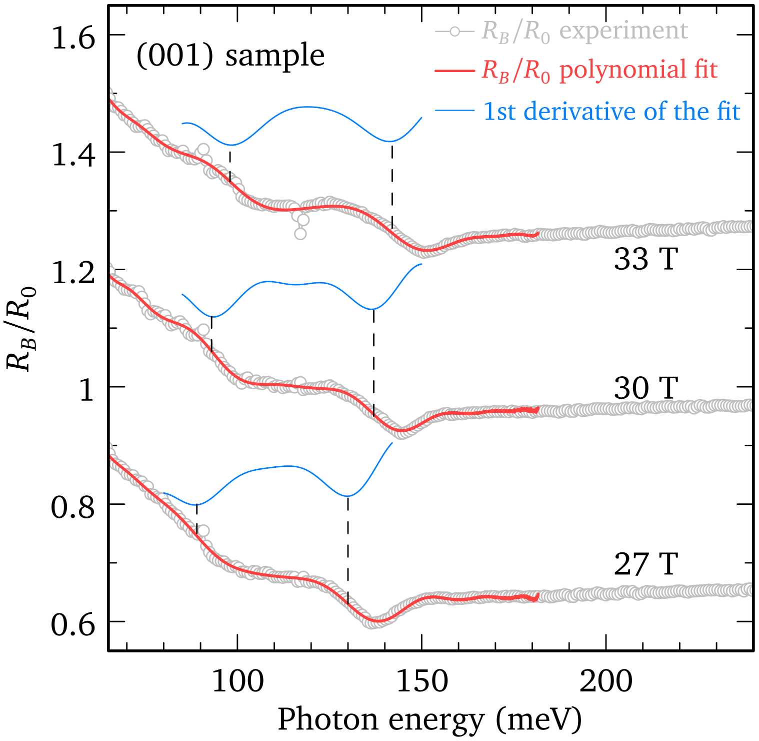


Fig. S7. Relative magneto-reflectivity spectra of the (001)-oriented sample taken at $B = 27, 30$ and 33 T (gray circles), fitted using a high-order polynomial function (red curves). The points of inflections, associated with the position of two CR modes, are taken as minima in the first derivative of the polynomial fit (blue curves).

Even though these additional data and the detailed analysis provide us with compelling evidence for the existence of the satellite lines, we remain conservative in our conclusions and denote their existence in our manuscript as *likely* but still not fully confirmed. Their existence merely gives a supporting argument in the interpretation of our data. The main conclusions are drawn based on the analysis of the clearly resolved main CR modes.

## MAGNETO-TRANSPORT CHARACTERIZATION OF THE STUDIED SAMPLES

$Cd_3As_2$ samples studied in our (magneto-)optical experiments were also characterized using the low-field magneto-transport technique. The electrical contacts were deposited using silver paste, which allowed us to probe the longitudinal magneto-resistance $R_{xx}(B)$ in a four-contact configuration. Further quantities, such as resistivity or carrier mobility, could not be deduced with a sufficient precision due to fairly irregular shape of samples, showing only one well-defined facet explored in our reflectivity study. The magnetic field was always applied perpendicular to the optical facets.

A summary of results from the (001)-oriented sample is presented in Figs. S8a-c. In line with previous experiments performed on samples from the same source [14], the longitudinal magneto-resistance $R_{xx}$ increases almost linearly with $B$ in the range of applied magnetic fields. Shubnikov-de Haas oscillations emerge in the background-removed data $\Delta R_{xx}(B)$ at $B \approx 2$ T (inset of Fig. S8a). They imply a single dominant oscillation frequency, $B_f \approx 37$ T, obtained when a fast Fourier transformation is applied to $\Delta R_{xx}(1/B)$, see Fig. S8b.

The deduced frequency $B_f \approx 37$ T perfectly matches our expectations based on the analysis of the optical data. The Fermi surface cross section of an ideal conical band $A = \pi E_F^2/(v^2\hbar^2)$ yields the oscillation frequency $B_f = \hbar A/(2\pi e) = E_F^2/(2e\hbar v^2)$. Taking the Fermi energy estimated for the (001)-oriented sample from the onset of interband absorption, $E_F^{001} \approx 200$ meV, and the band velocity, $v = 0.93 \times 10^6$ m/s, deduced from our CR modes, we obtain $B_f \approx 35$ T.

The damping of the quantum oscillations with temperature (the inset of Fig. S8a), which was analyzed using the standard Lifshitz-Kosevich formalism, brings another consistency check of our interpretation. A closer look at the damping of the amplitude at $B = 6.6$ T (Fig. S8c) implies the effective mass at the Fermi level of $m_{001} = 0.036m_0$.

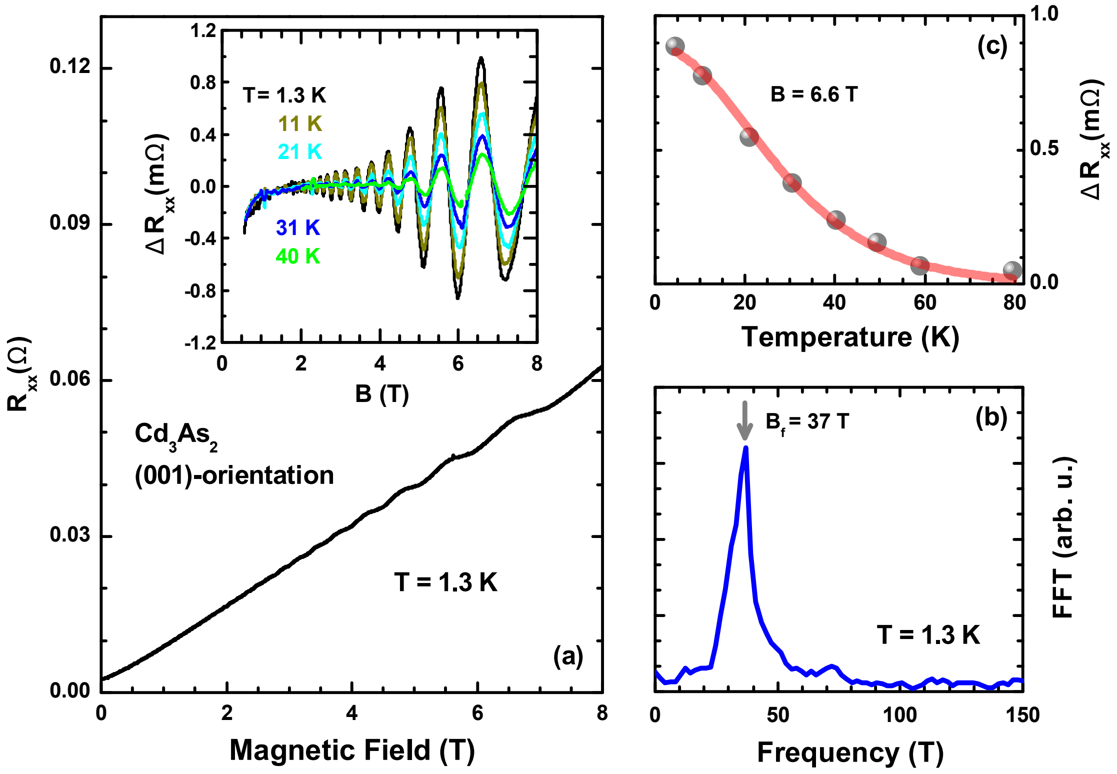


Fig. S8. The results of magneto-transport experiments performed on (001)-oriented sample. (a) Longitudinal magneto-resistivity $R_{xx}(B)$ measured at $T = 1.3$ K with quantum oscillations superimposed on nearly linear in $B$ background. The background-removed longitudinal resistivity traces $\Delta R_{xx}(B)$ measured at $T = 1.3, 11, 21, 31$ and 40 K are plotted in the inset. (b) a fast Fourier-transform of $\Delta R_{xx}(1/B)$ showing a clear periodicity of the observed oscillations in $1/B$ with a dominant frequency of $B_f = 37$ T. (c) Temperature dependence of the $\Delta R_{xx}$ amplitude at $B = 6.6$ T, implying the effective mass $m \approx 0.036 m_0$ at the Fermi level.

This agrees well with the effective mass expected theoretically, $m = E_F/v^2 = 0.041 m_0$, as well as that estimated from the plasma edge splitting at low magnetic fields, $m_{001} = 0.04 m_0$ (Fig. S4a).

In contrast to the (001)-oriented sample, the magneto-transport experiments carried out on the (112)-oriented sample did not bring any conclusive results. The main obstacle was preparing reliable ohmic electrical contacts for this low doped sample, where the carrier density estimated from the optical conductivity is as low as $n \sim 10^{17}$ cm$^{-3}$.

## INFLUENCE OF THE SPIN-ORBIT COUPLING STRENGTH

In the main part of the manuscript, the strength of the spin-orbit coupling in $Cd_3As_2$ was fixed at the value known for another arsenic-based semiconductor InAs, $\Delta = 400$ meV. Due to the limited space, we did not discuss in detail its influence on the presented modeling. Here we show that a reasonable variation of $\Delta$ does not imply any dramatic changes in the theoretically calculated positions of CR modes. We illustrate this in Fig. S9, where the experimentally deduced CR energies are plotted against their theoretically expected positions for particularly weak and strong values of $\Delta$. The velocity parameter was kept constant at $v = 0.93 \times 10^6$ m/s in these calculations. We may also note that the zero-field response of $Cd_3As_2$ is consistent with the spin-orbit coupling close to 400 meV or lower. Higher values would, according to the formula (S24), suppress the theoretically expected strength of the interband absorption in the middle infrared range and worsen agreement with our experimental data (in Fig. 1b in the main text).

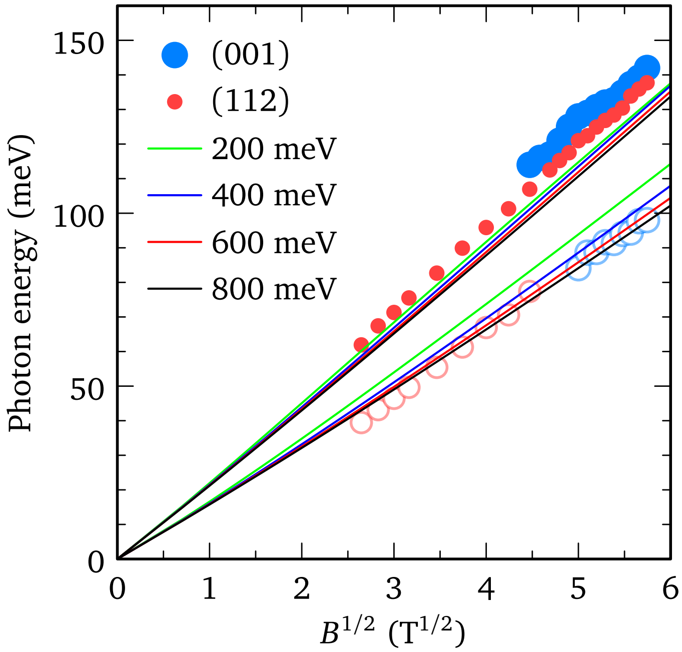


Fig. S9. The fan chart of observed CR modes in the (001)- and (112)-oriented sample compared to theoretically expected positions calculated within the gapless Kane model for various strength of the spin-orbit coupling $\Delta = 200, 400, 600$ and 800 meV while keeping the velocity parameter $v = 0.93 \times 10^6$ m/s constant.

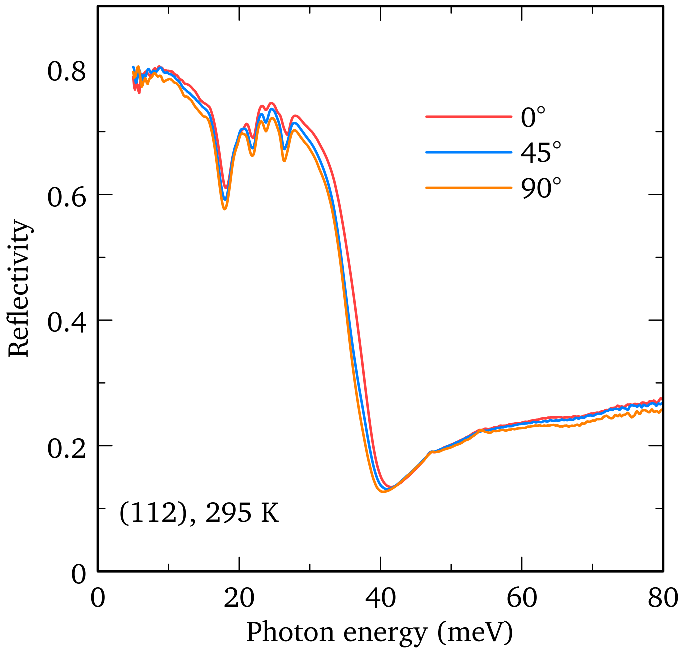


Fig. S10. Room-temperature reflectivity spectra of the (112)-oriented sample measured with linearly polarized radiation. Nearly identical response for three different orientations of the light polarization plane, encompassing two principal axes separated by 90°, implies very high isotropy of the optical response of $Cd_3As_2$. A gold mirror (not in-situ overcoating technique) was used as a reference for reflectivity measurements presented in this figure.

## REFLECTIVITY OF THE (112)-ORIENTED SAMPLE – ANISOTROPY OF THE OPTICAL RESPONSE

To estimate the degree of anisotropy in $Cd_3As_2$, we have performed a polarization-dependent measurement of the reflectivity for the (112)-oriented sample. In principle, the (112) facet may be optically anisotropic. The polarization

plane was rotated with respect to an arbitrarily chosen axis on the sample surface. Fig. S10 shows the spectra obtained for two principal optical axes, separated by 90°, and an angle in between. The shift in the plasma edge is close to 1 meV. This experiment provides us with another piece of evidence for high isotropy of the electronic bands in $Cd_3As_2$.

* milan.orlita@lncmi.cnrs.fr

[1] J. Bodnar, in *Proc. III Conf. Narrow-Gap Semiconductors, Warsaw*, edited by J. Raułuszkiewicz, M. Górska, and E. Kaczmarek (Elsevier, 1977) p. 311.
[2] H. Kildal, Phys. Rev. B **10**, 5082 (1974).
[3] E. O. Kane, J. Phys. Chem. Solids **1**, 249 (1957).
[4] M. Orlita, D. M. Basko, M. S. Zholudev, F. Teppe, W. Knap, *et al.*, Nature Phys. **10**, 233 (2014).
[5] P. R. Wallace, phys. stat. sol. (b) **92**, 49 (1979).
[6] M. König, S. Wiedmann, C. Brüne, A. Roth, H. Buhmann, L. W. Molenkamp, X.-L. Qi, and S.-C. Zhang, Science **318**, 766 (2007).
[7] P. E. C. Ashby and J. P. Carbotte, Phys. Rev. B **87**, 245131 (2013).
[8] A. R. Wright and R. H. McKenzie, Phys. Rev. B **87**, 085411 (2013).
[9] A. Raoux, M. Morigi, J.-N. Fuchs, F. Piéchon, and G. Montambaux, Phys. Rev. Lett. **112**, 026402 (2014).
[10] M. O. Goerbig, G. Montambaux, and F. Piéchon, EPL (Europhysics Letters) **105**, 57005 (2014).
[11] M. N. Ali, Q. Gibson, S. Jeon, B. B. Zhou, A. Yazdani, and R. J. Cava, Inorganic Chemistry **53**, 4062 (2014).
[12] H. Schleijpen, M. von Ortenberg, M. Gelten, and F. Blom, Int. J. Infrared Milli. **5**, 171 (1984).
[13] E. D. Palik and J. Furdyna, Rep. Prog. Phys. **33**, 1193 (1970).
[14] T. Liang, Q. Gibson, M. N. Ali, M. Liu, R. J. Cava, and N. P. Ong, Nature Mater. **14**, 280 (2015).
